# Supplementary material for: HEX: Humanoid-Aligned Experts for Cross-Embodiment Whole-Body Manipulation
Source: arXiv:2604.07993 source file (2026-10-22)
Supplement: Supplementary file 1 [file 6_appendix.tex]

\appendix

\setcounter{figure}{0}
\setcounter{table}{0}
\setcounter{equation}{0}

\section*{Appendix}
